# Supplementary material for: HammerHead: Leader Reputation for Dynamic Scheduling
Source: arXiv:2309.12713 source file (2023-09-22)
Supplement: Supplementary file 1 [file appendix.tex]

\label{sec:appendix}
\subsection{Theoretical Solution for Guaranteed Liveness}

\paragraph{Discussion on making the simplified protocol live:} In order for the simplified protocol to be shown live, the call to Bullshark would need to change, so that honest validators keep checking whether they have some new intermediate vertex to commit.
Specifically, an honest validator $P_i$ that has its previously committed anchor be $v_r$ and is currently in round $r'$, would keep checking whether it can commit some vertex for round $r_m\in(r,r']$. If they can commit, they would commit, potentially update the schedule, and continue to commit vertices. This idea would lead to liveness after GST because even the slower honest validators would be able to keep the schedule ``up-to-date'', i.e. they would be able to quickly recover, from committing the intermediate missing vertices they would newly receive and updating their schedules accordingly.
%In the good case all validators will switch from $S$ to $S'$ within a small time bounds (less than the time for the fast validators to move to $S''$). Hence if this happens the above proof holds. \lef{not sure why this is resposive, it actually is synchronous since to work we need every validator to get the new schedule within $K+1$ rounds}
\giorgos{I am thinking about this solution. Specifically, what exactly is the argument on how we achieve liveness now, while we did not before. So, before, assume that we have an honest validator, who is $f$ schedules behind.  }

\paragraph{Advanced (Theoretical) solution for guaranteed liveness.} The challenge of the previous solution is that in asynchrony each validator can in principle be in a different schedule. For this, we would need to compute new schedules, considering that all active schedules should have an $f+1$ overlap of validators. This means that we might not be able to swap out all validators from the $B$ set. All schedules are active from the beginning of the epoch until we can deactivate them.

\paragraph{Deactivating a schedule.} For liveness we need to give enough “points of liveness” to all active schedules. To achieve this all active schedules need to have f+1 leaders in common. \giorgos{I believe trying to solve this optimally is NP-hard, I think it becomes related to Set Cover (but haven't reduced it yet), so in practice with a heuristic we would get closer to the restrictions even faster.}
\begin{definition}[Pairwise Restriction Problem]
    Let $S_0$ be an $n$-vector containing $n=3f+1$ elements from $[n]$ (repetitions allowed). Let $\mathbf{S}=\{S_i\}_{i=0,\dots,m-1}$ be a sequence of $n$-vectors that are \emph{pairwise restricted}, i.e. there exist at least $f+1$ positions $p$ s.t. for every $i,j\in[m]$, $S_i[p]=S_j[p]$.
    The optimization problem $\mathsf{PR}(\mathbf{S}, n)$ is defined as: Given such a sequence $\mathbf{S}$ of pairwise restricted $n$-vectors, output the $n$-vector $S_m$ that differs from $S_{m-1}$ in as many positions as possible (but not more than $f$ many), while also $S_m$ is pairwise restricted with all $S_i\in\mathbf{S}$.\giorgos{If you have any ideas to simplify the potential problem to be shown NP-hard, let me know.}
\end{definition}

\giorgos{More updates on this: I was trying to reduce clique to the respective decision problem, but we have too many constraints. Because of that, it seems to me that a graph problem might be a harder starting point, so I will think about SAT or IP. }

The problem can be formulated as an optimization program.
For each $j\in{0,\dots,m}, i,p\in[n]$ let $X^j_{i,p}\in\{0,1\}$ be 1 iff the position $p$ of the vector $j$ has value $i$. Then, the problem takes the form:
\begin{align*}
    \min                  & \sum_{i,p} \big( X^m_{i,p}\cdot X^{m-1}_{i,p}\big)     \\
    \text{s.t.}           & \sum_{i,p}\big( X^m_{i,p}\cdot X^{m-1}_{i,p}\big)\le f \\
    \forall k,l\in\{0,m\} & \sum_{i,p}\big( X^l_{i,p}\cdot X^k_{i,p}\big)\ge f+1   \\
    \forall p,j           & \sum_{i} X^j_{i,p} = 1                                 \\
    \forall i,p,j         & X^j_{i,p} \in \{0,1\}
\end{align*}

To decouple the products and make the program linear, we can use the known technique of introducing one new variable for each product. Specifically, for each product $X^l_{i,p}\cdot X^k_{i,p}$ we introduce $Z^{k,l}_{i,p}$ such that:
\begin{align*}
    Z^{k,l}_{i,p} & \ge X^l_{i,p}+ X^k_{i,p} -1 \text{ \giorgos{1 iff both are 1, 0 else}} \\
    Z^{k,l}_{i,p} & \le X^l_{i,p}                                                          \\
    Z^{k,l}_{i,p} & \le X^k_{i,p}                                                          \\
    Z^{k,l}_{i,p} & \in \{0,1\}
\end{align*}
Similarly, the optimization function becomes $\min \sum_{i,p} Z^{m-1,m}_{i,p}$.
Since we have at least all the pairings be \newline \paragraph{Small example to get intuition:} Assume that we want to change up to 3 leaders from the schedule, so the smallest such example is for $n=10$.

As the number of schedules increases, this becomes more and more restrictive, which is why we provide a way to deactivate a schedule.

Every validator includes as extra metadata on their DAG blocks a schedule ID that specifies the schedule they are currently following (an integer value similar to “current-view”). When a leader commits, we look at the highest-round block of every party to see which schedule they were following. If $2f+1$ parties have advanced after a schedule we can deactivate it and stop providing legacy support for liveness, hence we now only require the $f+1$ leaders to be in common of the active schedules. In practice, these active schedules will be forced by this constraint to be only two.
The algorithm for switching leaders can be as follows:
\begin{enumerate}
    \item Every time a new schedule is initialized there is a vector of $3f+1$ slots tagged with static, leader-id.
    \item To initialize the new schedule go to the oldest active schedule and permute the leader-ids to generate the new schedule. There should always be $f+1$ static leader-ids on the oldest schedule.
    \item Propagate the new schedule to all other active schedules, updating the slots that changed with the new leader-id and a dynamic tag.
    \item When a schedule is deactivated, garbage collect it and always remember which is the oldest active schedule.
\end{enumerate}
